# Supplementary material for: Understanding Road Layout from Videos as a Whole
Source: arXiv:2007.00822 source file (2020-07-02)
Supplement: Supplementary file 1 [file supp.tex]

%\section{Introduction}
%This supplemental material contains the following details that we could not include in the main paper due to space restrictions: 1) Feature aggregation, 2) Implementation details,  3) IoU metric and 4) m ore results on NuScenes~\cite{sam:NuScenes18a}. Video example on KITTI test set can be found in the attached .avi file.

This supplemental material contains the following details that we could not include in the main paper due to space restrictions:
\begin{itemize}
\item {\bf (Sec.~\ref{sec:supp_fa})} Details on feature aggregation
\item {\bf (Sec.~\ref{sec:supp_impl})} Implementation details
\item {\bf (Sec.~\ref{sec:supp_iou})} The IoU metric for evaluation
\item {\bf (Sec.~\ref{sec:supp_res_nuscenes})} Results on NuScenes~\cite{sam:NuScenes18a}
\item {\bf (Sec.~\ref{sec:supp_video})} Result video on KITTI data
\end{itemize}

\section{Details on feature aggregation}
\label{sec:supp_fa}
We introduce our Feature transform module (FTM) in Sec. 3.2.1 of the main paper and utilize a summation to aggregate the features from consecutive frames.
Although simple, the summation is very general in a sense that it enables our model to aggregate frames from an arbitrary amount of other frames.
%This design is for better generality of our method.
While we demonstrate FTM with two consecutive frames in the main paper (enabling an online system), we can easily extend our model by aggregating features from multiple frames that are further away or even from future frames in offline settings.
%Specifically, we can easily extend our model by aggregating features from frames that are further away or even from future frames in offline settings.
This may not be said for other operations.
For instance, feature concatenation changes the internal feature dimensions (and thus network architecture) if information from more frames are available; max pooling cannot guarantee information propagation.
%\bing{How about other operations? Like, feature concatenation can also be extended for more frames, but less easily since network architecture needs to change? What does "easily" mean? How about doing a max pooling to merge the two feature map into one?} 
Moreover, our FTM can be readily extended for multiple feature maps at different spatial scales, which can potentially further improve the performance.
%\bing{max pooling also can?}

\section{Implementation details}
\label{sec:supp_impl}
\subsection{Model learning and inference}
We use ADAM~\cite{sam:Kingma15a} to minimize $\lossSupReal$ and estimate the parameters of our neural network.
To effectively train the entire model, we first train a $basic$ model defined as follows: %with the loss defined in Eq.~\ref{eq:full_loss}. The single image based model is defined below:
\begin{equation}
\begin{split}
    \sa^t = & (\nnAttr \circ \nnFeat_{j} \circ \nnFeat_{i}) (\bevmap^t). \\
\end{split}
\label{eq:singleimage_NN}
\end{equation}
This model receives $\bevmap^t$ as input and makes predictions individually on each frame.
We then add an LSTM, creating a new model denoted as $blstm$
\begin{equation}
\begin{split}
    \sa^t = & (\nnAttr \circ \nnFeat_{lstm} \circ \nnFeat_{j}) (\nnFeat_{i}(\bevmap^t),\nnFeat_{i}(\bevmap^{t-1})) \;, \\
\end{split}
\label{eq:LSTM_NN}
\end{equation}
which we train with pre-trained parameters for the functions $\nnAttr$, $\nnFeat_{j}$ and $\nnFeat_{i}$.
Finally, we add the FTM and fine-tune the full model (with parameters pre-trained as above).
Details of our $basic$ and $blstm$ models can be found in the experiment section of the main paper.

In training, we set the learning rate to $1e\text{-}4$ for the model $basic$, the batch size to 26, and update the model for 50k iterations. The $blstm$ model as well as our full network are then trained with a batch size of 20 for 30k iterations and a learning rate of $1e\text{-}5$.

\begin{table}\centering\small
\setlength{\belowcaptionskip}{-0.4cm}
  %\begin{tabular}{l|cccc}
%  \hline
%              & \multicolumn{4}{c}{NuScenes~\cite{sam:NuScenes18a}} \\
%  \hline
%  Method      & Accu.-Bi. $\uparrow$ &  Accu.-Mc. $\uparrow$ & MSE $\downarrow$ & IOU $\uparrow$ \\
%  \hline\hline
%  BEV~\cite{Wang_2019_CVPR}          & .846    & .485      & .073 & .217\\
%  H-BEV+DA~\cite{Wang_2019_CVPR}+GM & \textbf{.877} & .496 & .032 & \textbf{.326} \\
%  \hline
%  BEV-C          & .856    & .471      & .069 & .211\\
%  BEV-J        & \textbf{.872}      & .486      & .036 & .230\\
%  BEV-J-O      & .858      & \textbf{.543}      & .027 & .313\\  
%  \hline
%  +LSTM        & .859 & .536  & \textbf{.023}  &  .311  \\
%  +LSTM+FTM      & .863 & \textbf{.547} & \textbf{.023} & \textbf{.328} \\    
%  \hline
%\end{tabular}

\begin{tabular}{l|ccc}
  \hline
              & \multicolumn{3}{c}{NuScenes~\cite{sam:NuScenes18a}} \\
  \hline
  Method      & Accu.-Bi. $\uparrow$ &  Accu.-Mc. $\uparrow$ & MSE $\downarrow$ \\
  \hline\hline
  BEV~\cite{Wang_2019_CVPR}          & .846    & .485      & .073\\
  H-BEV+DA~\cite{Wang_2019_CVPR}+GM & \textbf{.877} & .496 & .032\\
  \hline
  BEV-C          & .856    & .471      & .069\\
  BEV-J        & \textbf{.872}      & .486      & .036\\
  BEV-J-O      & .858      & \textbf{.543}      & .027\\  
  \hline
  +LSTM        & .859 & .536  & \textbf{.023}\\
  +LSTM+FTM      & .863 & \textbf{.547} & \textbf{.023}\\    
  \hline
\end{tabular}
  \vspace{-0.2cm}
  \caption{Full results on NuScenes dataset.}
  \label{tbl:nusceneresult}
\end{table}

\begin{table}\centering\small
\setlength{\belowcaptionskip}{-0.4cm}
  \begin{tabular}{l|cc}
  \hline
              & \multicolumn{2}{c}{NuScenes~\cite{sam:NuScenes18a}} \\
  \hline 
  Method      &  seman.$\downarrow$& temp.$\downarrow$ \\
  \hline
  BEV~\cite{Wang_2019_CVPR} & 1.09 & 1.27\\
  H-BEV-DA~\cite{Wang_2019_CVPR}+GM&  0.07 & 0.52 \\                  
  \hline
  BEV-J-O &  0.52& 1.14\\
  \hline
  +LSTM+FTM & 0.10 & 0.51\\
\end{tabular}
  \vspace{-0.2cm}
  \caption{Consisency measurements on NuScenes dataset.}
  \label{tbl:nusceneconsistency}
\end{table}

\subsection{Scene Attributes}
As mentioned in paper, we exactly follow the scene parameters defined in~\cite{Wang_2019_CVPR}. Specifically, we describe them in more details in Tab.~\ref{tbl:scene_attributes}.

\begin{table}\centering\small
  \begin{tabular}{l|p{6.2cm}}
    \hline
    ID                     & Description\\
    \hline\hline
    \textcolor{green}{\textbf{B1}}  & Is the main road curved? \\
    \textcolor{green}{\textbf{B2}}  & Is the main road a one-way? \\
    \textcolor{green}{\textbf{B3}}  & Does the main road have a delimiter?\\
    \textcolor{green}{\textbf{B4}}  & Is there a delimiter between road and side walks?\\
    \textcolor{green}{\textbf{B5}}  & Does a sidewalk exist on the left of the main road?\\
    \textcolor{green}{\textbf{B6}}  & Does a sidewalk exist on the right of the main road?\\
    \textcolor{green}{\textbf{B7}}  & Does a crosswalk exist before the intersection?\\
    \textcolor{green}{\textbf{B8}}  & Does a crosswalk exist after the intersection?\\
    \textcolor{green}{\textbf{B9}}  & Does a crosswalk exist on the left side road of the intersection? \\
    \textcolor{green}{\textbf{B10}} & Does a crosswalk exist on right side road of the intersection?\\
    \textcolor{green}{\textbf{B11}} & Does a crosswalk exist on the main road w/o intersection?\\
    \textcolor{green}{\textbf{B12}} & Does a  left side road exist?\\
    \textcolor{green}{\textbf{B13}} & Does a right side road exist?\\
    \textcolor{green}{\textbf{B14}} & Does the main road end after the side roads?\\
    \hline
    \textcolor{green}{\textbf{M1}}  & Number of lanes on the left of the ego-lane (maximum 6)\\
    \textcolor{green}{\textbf{M2}}  & Number of lanes on the right of the ego-lane (maximum 6)\\
    \hline
    \textcolor{green}{\textbf{C1}}  & Rotation angle of the main road (\eg, when car makes a turn)\\
    \textcolor{green}{\textbf{C2}}  & Width of the right side road \\
    \textcolor{green}{\textbf{C3}}  & Width of the left side road \\
    \textcolor{green}{\textbf{C4}}  & Width of a delimiter on the main road\\
    %\textcolor{OrangeRed}{\textbf{C5}}    & (NOT ANNOTATED?) Width of delimiter on right side road \\
    %\textcolor{OrangeRed}{\textbf{C6}}    & (NOT ANNOTATED?) Width of delimiter on the left side road \\
    \textcolor{green}{\textbf{C5}}  & Distance to right side street \\
    \textcolor{green}{\textbf{C6}}  & Distance to left side street \\
    \textcolor{green}{\textbf{C7}}  & Distance to crosswalk on the main road without intersections \\
    %\textcolor{OrangeRed}{\textbf{C10}}   & (NOT ANNOTATED?) Width of sidewalk on the main road \\
    \textcolor{green}{\textbf{C8}}  & Width of delimiter between main road and sidewalk \\
    \textcolor{green}{\textbf{C9}}  & Curve radius of the main road \\
    \textcolor{red}{\textbf{C10-22}}& Lane widths ($6 \times 2 + 1$) \\
    \hline
  \end{tabular}
  \caption{The list of all our scene attributes $\sa$ is divided into groups as in the main paper: binary $\saBin$, multi-class $\saMc$ and continuous $\saReg$.  Each attribute is assigned an ID preceded by its group ID (B, M or C).  The color of the ID indicates if manual annotation on real data exists (\textcolor{green}{green}).  Attributes only available in simulation are marked \textcolor{red}{red}.}
  \label{tbl:scene_attributes}
\end{table}

\paragraph{Discretize continuous attributes}
Formulating continuous attribute prediction as a regression problem in the discretized space permits multiple modes in the final prediction. This can be further leveraged by subsequent graphical models, if available, as the unary term to find feasible solutions that avoid conflicts among different attributes.

\subsection{Consistency}
\begin{itemize}
\item {\em Semantic consistency:} we report the average conflicts in attribute predictions. % w.r.t. their semantic meanings. 
Since no constraints are enforced explicitly in models, it is likely that they output infeasible predictions, e.g. one binary variable predicts [no sideroads] but another one predicts [crosswalk on the left side of intersection]. 
%In this case, We count one infeasible prediction 
%\sam{I'm not sure if it is clear to the reader what infeasible means here since we did not explain the graphical model or the scene model} 
%as a conflict. %More details can be found in~\cite{Wang_2019_CVPR}.
%Since no constraints are enforced explicitly in models, it is likely that they output infeasible predictions, e.g. one model predicts that there exists no sideroads but has a crosswalk on the left side of intersection. 
In this case, we count a conflict if the predicted attributes are node feasible and report the average number of conflicts as our semantic consistency measurements.
\item {\em Temporal consistency:} we also report the average number of changes in our prediction. Specifically, if the prediction for one attribute changes in consecutive frame, we count it as a change. Intuitively, a good model should have lower number in this measurement. Note that we only consider the binary and multiclass tasks in this measurement. Also, since the predictions can be consistently wrong over time, consistency itself cannot replace accuracy.  
\end{itemize}

\section{IoU measurement}
\label{sec:supp_iou}
Here, we provide more explanations on our evaluation metric. We would like to point out that the Intersection over Union (IoU) score reported in our paper is different from what has been reported in semantic segmentation literature. In short, the two semantic maps to compute IoU are both rendered from a set  of parametric attributes, rather than per-pixel predicted as usually done.
%More specifically, instead of predicting the non-parametric semantic top-view map directly, we propose to predict the scene attributes in top-view and render the scene w.r.t. predicted results. After mapping both the predicted attributes and ground-truth ones to top-view, we can then compute their IoU score over four background classes, e.g. road, lane boundary, crosswalk and sidewalk. 

%\sam{Why do we always mention traditional IoU? IoU itself is the same, but only how we get the semantic maps is different. And the original reason we did this in the CVPR paper was only to entangle the attributes with the renderer to see the impact of certain parameters to the final scene output.}

Similar to~\cite{Wang_2019_CVPR}, our IoU has two differences compared to the IoU of a typical semantic segmentation task: 1) the semantic top-view maps are obtained with a rendering function, which is highly nonlinear and cannot be directly optimized; 2) the rendered semantic top-view maps entangle all three types of attributes together and their impact on IoU varies a lot. For instance, predicting the number of lanes on the left incorrectly by one has a bigger impact than getting the distance to a crosswalk wrong by one meter. 

% \todo{We should cite the CVPR19 paper that introduces this metric.}

\section{Results on nuScenes}
\label{sec:supp_res_nuscenes}
We report more results on the nuScenes~\cite{sam:NuScenes18a} dataset in Tab.~\ref{tbl:nusceneresult} and Tab.~\ref{tbl:nusceneconsistency}, which we could not fit into the main paper due to the space limitation. Note that compared to the SOTA model H-BEV+DA+GM from~\cite{Wang_2019_CVPR}, we use far less human annotations. In their experiments, Wang~\etal have 3486 and 1042 images for training and testing, respectively. While in our case, we have 1165 images for training and 348 for testing. This is because we remove those frames where the car stops, since there is no additional temporal information to utilize and thus not relevant for our investigation. More importantly, \cite{Wang_2019_CVPR} utilized 50k additional synthetic images to assist training and adopted a graphical model for post processing, which we do not use in our approach.

As can be seen in Tab.~\ref{tbl:nusceneresult}, our proposed method outperforms the $basic$ BEV model in all metrics. This demonstrates the effectiveness of our proposed input representation as well as the LSTM/FTM module. Compared to the SOTA method H-BEV+DA+GM~\cite{Wang_2019_CVPR}, we show that our proposed model can achieve better performance in almost all metrics, except the binary class accuracy where we are slightly worse. Note that although our binary accuracy is worse ($1.4\%$ lower), the accuracy for multi-class scene attributes is much higher than SOTA ($4.9\%$ higher). Similarly, we show in Tab.~\ref{tbl:nusceneconsistency} that our input representation and the LSTM/FTM modules improve the prediction consistency over the baseline significantly, and can achieve comparable performance w.r.t. SOTA.

\section{Result video}
\label{sec:supp_video}
We also attach a video demonstration (see supple-video.avi for more details) of our method in this supplementary. As can be seen in the video, our predictions are quite smooth and are consistent with 3D object prediction results.
% \sam{Describe the video quickly. Write the filename.}
