# Supplementary material for: Understanding Road Layout from Videos as a Whole
Source: arXiv:2007.00822 source file (2020-07-02)
Supplement: Supplementary file 3 [file supp_nuscenes_accuracy.tex]

%\begin{tabular}{l|cccc}
%  \hline
%              & \multicolumn{4}{c}{NuScenes~\cite{sam:NuScenes18a}} \\
%  \hline
%  Method      & Accu.-Bi. $\uparrow$ &  Accu.-Mc. $\uparrow$ & MSE $\downarrow$ & IOU $\uparrow$ \\
%  \hline\hline
%  BEV~\cite{Wang_2019_CVPR}          & .846    & .485      & .073 & .217\\
%  H-BEV+DA~\cite{Wang_2019_CVPR}+GM & \textbf{.877} & .496 & .032 & \textbf{.326} \\
%  \hline
%  BEV-C          & .856    & .471      & .069 & .211\\
%  BEV-J        & \textbf{.872}      & .486      & .036 & .230\\
%  BEV-J-O      & .858      & \textbf{.543}      & .027 & .313\\  
%  \hline
%  +LSTM        & .859 & .536  & \textbf{.023}  &  .311  \\
%  +LSTM+FTM      & .863 & \textbf{.547} & \textbf{.023} & \textbf{.328} \\    
%  \hline
%\end{tabular}

\begin{tabular}{l|ccc}
  \hline
              & \multicolumn{3}{c}{NuScenes~\cite{sam:NuScenes18a}} \\
  \hline
  Method      & Accu.-Bi. $\uparrow$ &  Accu.-Mc. $\uparrow$ & MSE $\downarrow$ \\
  \hline\hline
  BEV~\cite{Wang_2019_CVPR}          & .846    & .485      & .073\\
  H-BEV+DA~\cite{Wang_2019_CVPR}+GM & \textbf{.877} & .496 & .032\\
  \hline
  BEV-C          & .856    & .471      & .069\\
  BEV-J        & \textbf{.872}      & .486      & .036\\
  BEV-J-O      & .858      & \textbf{.543}      & .027\\  
  \hline
  +LSTM        & .859 & .536  & \textbf{.023}\\
  +LSTM+FTM      & .863 & \textbf{.547} & \textbf{.023}\\    
  \hline
\end{tabular}
