# Supplementary material for: Understanding Road Layout from Videos as a Whole
Source: arXiv:2007.00822 source file (2020-07-02)
Supplement: Supplementary file 4 [file supp_nuscenes_consistency.tex]

\begin{tabular}{l|cc}
  \hline
              & \multicolumn{2}{c}{NuScenes~\cite{sam:NuScenes18a}} \\
  \hline 
  Method      &  seman.$\downarrow$& temp.$\downarrow$ \\
  \hline
  BEV~\cite{Wang_2019_CVPR} & 1.09 & 1.27\\
  H-BEV-DA~\cite{Wang_2019_CVPR}+GM&  0.07 & 0.52 \\                  
  \hline
  BEV-J-O &  0.52& 1.14\\
  \hline
  +LSTM+FTM & 0.10 & 0.51\\
\end{tabular}
